# Supplementary material for: Entity-Based Knowledge Conflicts in Question Answering
Source: arXiv:2109.05052 source file (2022-01-12)
Supplement: Supplementary file 1 [file appendix.tex]

\section*{Appendix}
\appendix
\section{Reproducibility}

\subsection{Generative Reader Model}

In this work, we leverage the T5 Salient Span Masking(SSM) fine-tuned models released by \citep{roberts2020much} with same hyper-parameters for training all Generative Reader models.

We used v3-128 TPU with TPU software version 2.4.1 and used Tensorflow \citep{tensorflow} version 2.4.1 to run all of our experiments.

\subsection{Training time}
We provide the time it took to fine-tune a particular model variant for 10k steps in Table.

\begin{table}[h]
    \centering
    \begin{tabular}{lr}
    \toprule
    \textbf{Model size} & Time (minutes)\\
        \midrule
        \abr{T5-SSM Small} & 20 \\
        \abr{T5-SSM Large} & 80  \\
        \abr{T5-SSM 3B} & 200  \\
        \abr{T5-SSM 11B} & 810 \\
        \bottomrule
    \end{tabular}
    \caption{Training times.}
    \label{tbl:model_size_vs_time}
    \vspace*{-.4cm}
\end{table}
